# Supplementary material for: Impact of surface reflectivity on the ultra-fast laser melting of silicon-germanium alloys
Source: arXiv:2303.15977 source file (2023-09-08)
Supplement: Supplementary file 1 [file Supplementary_Materials.pdf]

## Supporting Information for:

### Impact of the crystalline and liquid phases reflectivity on the ultra-fast laser melting of silicon-germanium alloys

Damiano Ricciarelli<sup>a\*</sup>, Richard Daubriac<sup>b</sup>, Giovanni Mannino<sup>a</sup>, Ioannis Deretzi<sup>a</sup>, Gaetano Calogero<sup>a</sup>, Giuseppe Fisicaro<sup>a</sup>, Remi Demoulin<sup>b</sup>, Fuccio Cristiano<sup>b</sup>, Paweł P. Michałowski<sup>c</sup>, Pablo Acosta-Alba<sup>d</sup>, Jean-Michel Hartmann<sup>d</sup>, Sébastien Kerdilès<sup>d</sup> and Antonino La Magna<sup>a\*</sup>

<sup>a</sup> CNR IMM, Z.I. VIII Strada 5, 95121 Catania, Italy

<sup>b</sup> LAAS, CNRS and Université de Toulouse, 7av. Du Col. Roche, 31400 Toulouse, France

<sup>c</sup> Łukasiewicz Research Network—Institute of Microelectronics and Photonics, Warsaw, Poland

<sup>d</sup> CEA-LETI, Minatec Campus, F-38054 Grenoble, France

Email: [damiano.ricciarelli@imm.cnr.it](mailto:damiano.ricciarelli@imm.cnr.it), [antonino.lamagna@imm.cnr.it](mailto:antonino.lamagna@imm.cnr.it)

#### *EDX Ge composition profiles calibration by RBS dose measurements on strained Si<sub>1-x</sub>Ge<sub>x</sub> samples*

30 nm-thick pseudomorphic Si<sub>1-x</sub>Ge<sub>x</sub> layers were grown by RPCVD (Reduced Pressure Chemical Vapor Deposition) in an Epsilon 3200 tool from ASM, on p-type (100) bulk silicon 300 mm wafers. The bulk Si substrates surfaces were first prepared with a 30 s HF (0.5%) / HCl wet cleaning in a SU-3100 cleaning system from SCREEN, and then, shortly after, with a H<sub>2</sub> bake (1100 °C, 2 min) in the CVD chamber, in order to remove the native oxide. After such a surface preparation, Si<sub>1-x</sub>Ge<sub>x</sub> layers were deposited at 550°C, 20 Torr, with SiH<sub>2</sub>Cl<sub>2</sub> and GeH<sub>4</sub> precursors. UV-NLA was performed with the same laser tool as described previously and similar environment conditions (room temperature, atmospheric pressure, constant incident N<sub>2</sub> flux). In this design of experiments, areas of 15 x 15 mm<sup>2</sup> were exposed to single laser pulses at various energy densities, ranging from 1.40 to 2.40 J/cm<sup>2</sup> (with variable incremental steps between 0.025 - 0.050 J/cm<sup>2</sup>). In this range of ED, all laser regimes can be studied, from sub-melt to complete melt of the 30 nm-thick Si<sub>1-x</sub>Ge<sub>x</sub> layers and above, into the Si underneath.

A dedicated study was devoted to the precise measurement of the final composition of the 30 nm-thick strained Si<sub>1-x</sub>Ge<sub>x</sub> layers by combining Scanning Transmission Electron Microscopy- Energy Dispersive X-ray spectroscopy (STEM-EDX) and Rutherford Backscattering Spectroscopy (RBS) measurements. STEM-EDX measurements were performed on cross-section lamellas, fabricated by Focused Ion Beam (FIB) in a Helios 450S Scanning Electron Microscope (SEM) from FEI. EDX mappings have been measured thanks to a Transmission Electron Microscope (TEM) JEM-ARM200F Cold FEG equipped with a EDX SDD CENTURIO-X detector from JEOL. X-ray signals in selected areas have been quantified via the Cliff and Lorimer factor method to extract Ge content profiles as function of depth. RBS is an effective technique to quantify precisely the composition inside thin films, without the use of reference sample. Thus, the Ge doses measured by RBS were used to finely calibrate the Cliff and Lorimer factor for each sample. The resulting Ge EDX profiles have been compared to Ge SIMS profiles made in the same samples. Due to small variations in the sputtering rate in regions where the Ge content is strongly varying, Ge SIMS profiles depth scales is underestimated. Based on STEM/TEM thickness measurements, a proper depth scale adjustment has been applied to these SIMS profiles. In the end, the corrected Ge SIMS and EDX profiles are in good accordance, which validates our EDX calibration by RBS measurements.

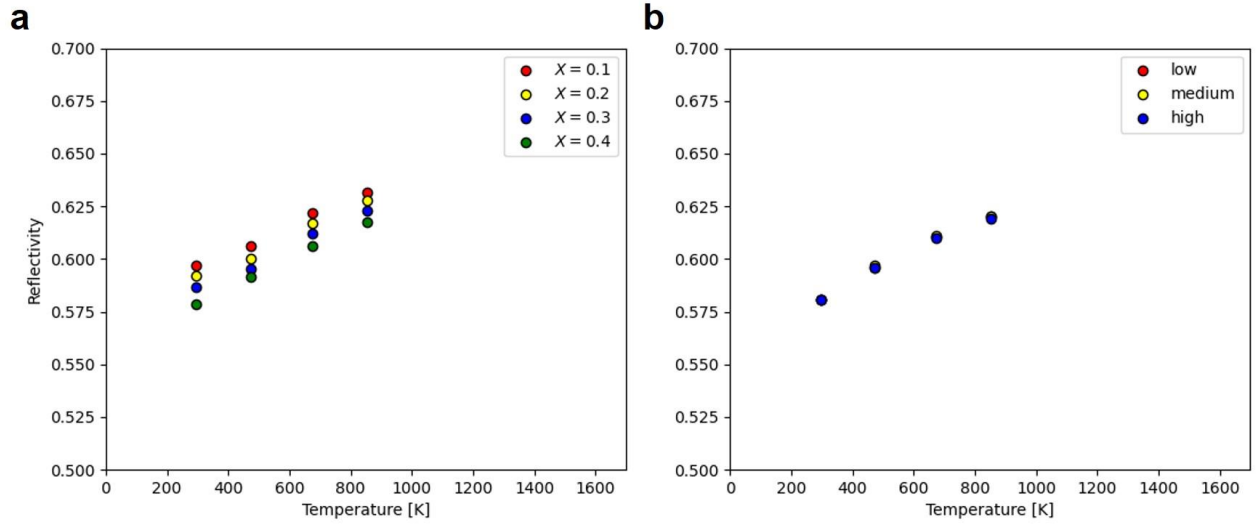

**Figure S1.** Reflectivity at a wavelength of 308 nm computed from dielectric functions for undoped (a) and doped (b) samples. For more details cf. main text.

**Table S1.** Real and imaginary part of dielectric functions of liquid silicon and germanium from [1].

|                    | $\Re$   | $\Im$  |
|--------------------|---------|--------|
| $\epsilon_{l, Si}$ | -15.734 | 10.126 |
| $\epsilon_{l, Ge}$ | -14.585 | 9.517  |

**Table S2.** Computed ED thresholds for relaxed and strained samples. Cf. main text for definition of the sample type and model.

| Sample                               | Computed ED threshold<br>[J cm <sup>-2</sup> ] |
|--------------------------------------|------------------------------------------------|
| Relaxed; X=0.24; $\Delta t = 160$ ns | 0.45                                           |
| Relaxed; X=0.58; $\Delta t = 160$ ns | 0.35                                           |
| Strained; X=0.2; $\Delta t = 146$ ns | 1.15                                           |
| Strained; X=0.4; $\Delta t = 146$ ns | 1.05                                           |
| Strained; X=0.2; $\Delta t = 160$ ns | 1.20                                           |
| Strained; X=0.3; $\Delta t = 160$ ns | 1.10                                           |

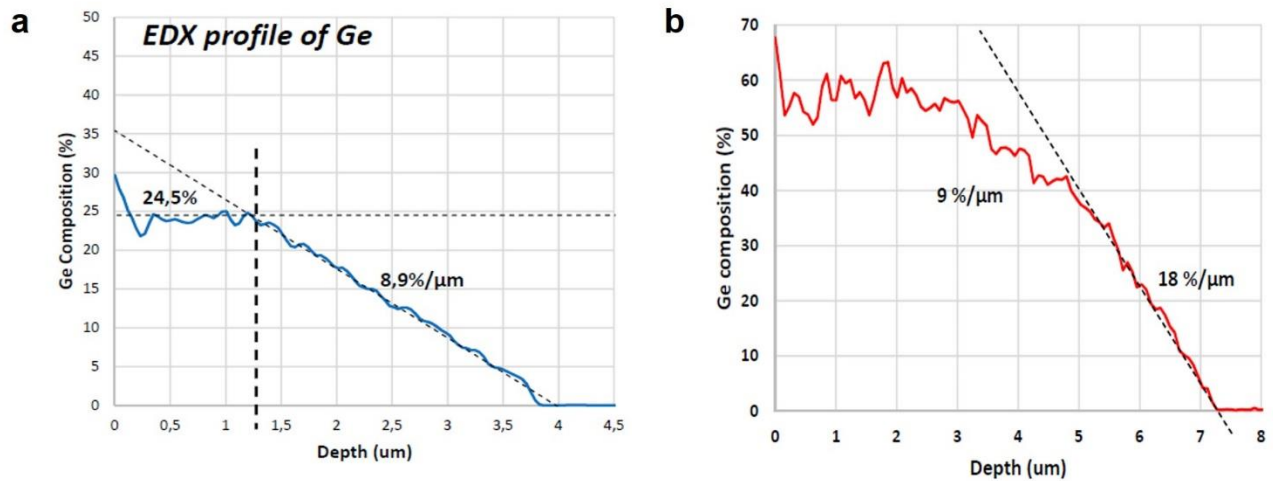

**Figure S2.** EDX germanium profiles measured for the as-deposited relaxed samples with alloy fractions of 0.24 (a) and 0.58 (b).

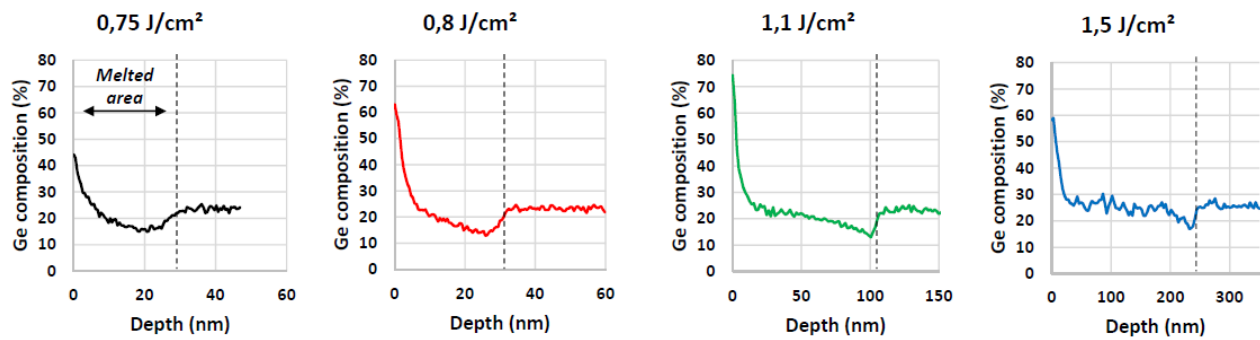

**Figure S3.** EDX germanium profiles obtained for the X=0.24 samples after laser irradiation.

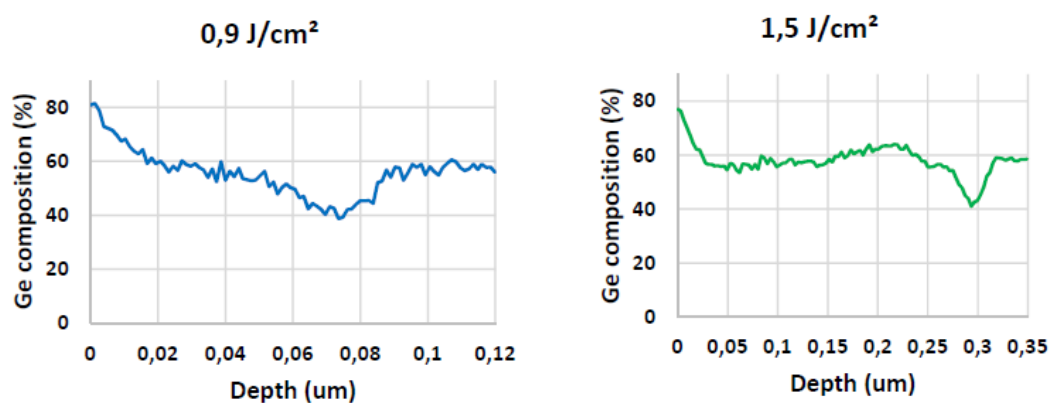

**Figure S4.** EDX germanium profiles obtained for the X=0.58 samples after laser irradiation.

**Table S3.** Melt depths obtained for X=0.24 relaxed samples, employing linear and quadratic T dependencies in the  $a(T)$  polynomial. Cf. main text.

| ED<br>[J / cm <sup>2</sup> ] | MD linear $\mathfrak{Z}(\epsilon_l)$<br>[nm] | MD quadratic $\mathfrak{Z}(\epsilon_l)$<br>[nm] | MD exp.<br>[nm] |
|------------------------------|----------------------------------------------|-------------------------------------------------|-----------------|
| 0.75                         | 25                                           | 26                                              | 25              |
| 1.10                         | 102                                          | 100                                             | 100             |
| 1.50                         | 224                                          | 218                                             | 238             |

**Table S4.** Melt depths obtained with calibration from EDX profiles for various alloy fraction and thickness of the Si<sub>1-x</sub>Ge<sub>x</sub> sample ( $a(T)$  calibrated parameters: **b1 = 0.8787; b2= -0.4159; c1=-496.7; c2=257.9**). Cf. main text.

| X    | ED<br>[J cm <sup>-2</sup> ] | MD<br>1300 nm<br>thick SiGe<br>[nm] | MD<br>3000 nm<br>thick SiGe<br>[nm] | MD<br>770 nm<br>thick SiGe<br>[nm] | MD<br>710 nm<br>thick SiGe<br>[nm] | MD exp.<br>[nm] |
|------|-----------------------------|-------------------------------------|-------------------------------------|------------------------------------|------------------------------------|-----------------|
| 0.20 | 0.75                        | -                                   | 22                                  | 23                                 | -                                  | 25              |
| 0.20 | 1.10                        | -                                   | 98                                  | 98                                 | -                                  | 100             |
| 0.20 | 1.50                        | -                                   | 219                                 | 219                                | -                                  | 238             |
| 0.24 | 0.75                        | 25                                  | -                                   | -                                  | -                                  | 25              |
| 0.24 | 1.10                        | 102                                 | -                                   | -                                  | -                                  | 100             |
| 0.24 | 1.50                        | 224                                 | -                                   | -                                  | -                                  | 238             |
| 0.50 | 0.90                        | -                                   | 77                                  | -                                  | 78                                 | 74              |
| 0.50 | 1.50                        | -                                   | 258                                 | -                                  | 258                                | 294             |
| 0.58 | 0.90                        | 84                                  | -                                   | -                                  | -                                  | 74              |
| 0.58 | 1.50                        | 277                                 | -                                   | -                                  | -                                  | 294             |

**Table S5.** Optimal  $\mathfrak{Z}(\epsilon_l)$  obtained for matching the various melt depths considering nominal concentration of the sample as initial X. ( $a(T)$  calibrated parameters: **b1 = 0.56023; b2= -0.17957; c1=-355.97; c2=155.91**). Cf. main text.

| X    | ED<br>[J cm <sup>-2</sup> ] | Optimal $\mathfrak{Z}(\epsilon_l)$ | $T_l$<br>[K] | MD exp.<br>[nm] |
|------|-----------------------------|------------------------------------|--------------|-----------------|
| 0.20 | 0.75                        | 8.5                                | 1652         | 25              |
| 0.20 | 1.10                        | 8.5                                | 1662         | 100             |
| 0.20 | 1.50                        | 10.1                               | 1703         | 238             |
| 0.50 | 0.90                        | 7.6                                | 1581         | 74              |
| 0.50 | 1.50                        | 10.7                               | 1651         | 294             |

**Table S6** Melt depths obtained for  $ED > 2.00 \text{ J cm}^{-2}$  for strained samples with a studied cut-off of the imaginary dielectric function expression. Cf. main text.

| <b>X</b> | <b>ED<br/>[J / cm<sup>2</sup>]</b> | <b>Pulse<br/>[ns]</b> | <b><math>\Im(\epsilon_i)</math><br/>cutoff</b> | <b>R<sub>i</sub><br/>cutoff</b> | <b>MD<br/>[nm]</b> | <b>MD exp.<br/>[nm]</b> |
|----------|------------------------------------|-----------------------|------------------------------------------------|---------------------------------|--------------------|-------------------------|
| 0.2      | 2.20                               | 146                   | 8.358                                          | 0.801                           | 43                 | 38                      |
| 0.2      | 2.40                               | 146                   | 8.358                                          | 0.801                           | 81                 | 81                      |

### References

1. Huet, K., et al., *Pulsed laser annealing for advanced technology nodes: Modeling and calibration*. Appl. Surf. Sci., 2020. **505**: p. 144470.
